# Supplementary material for: A Goal-Driven Survey on Root Cause Analysis
Source: arXiv:2510.19593 source file (2025-10-22)
Supplement: Supplementary file 1 [file 12appendix.tex]

\section{APPENDIX}\label{sec:appendix}

\begin{figure}[t]
    \centering
    \includegraphics[width=1\linewidth]{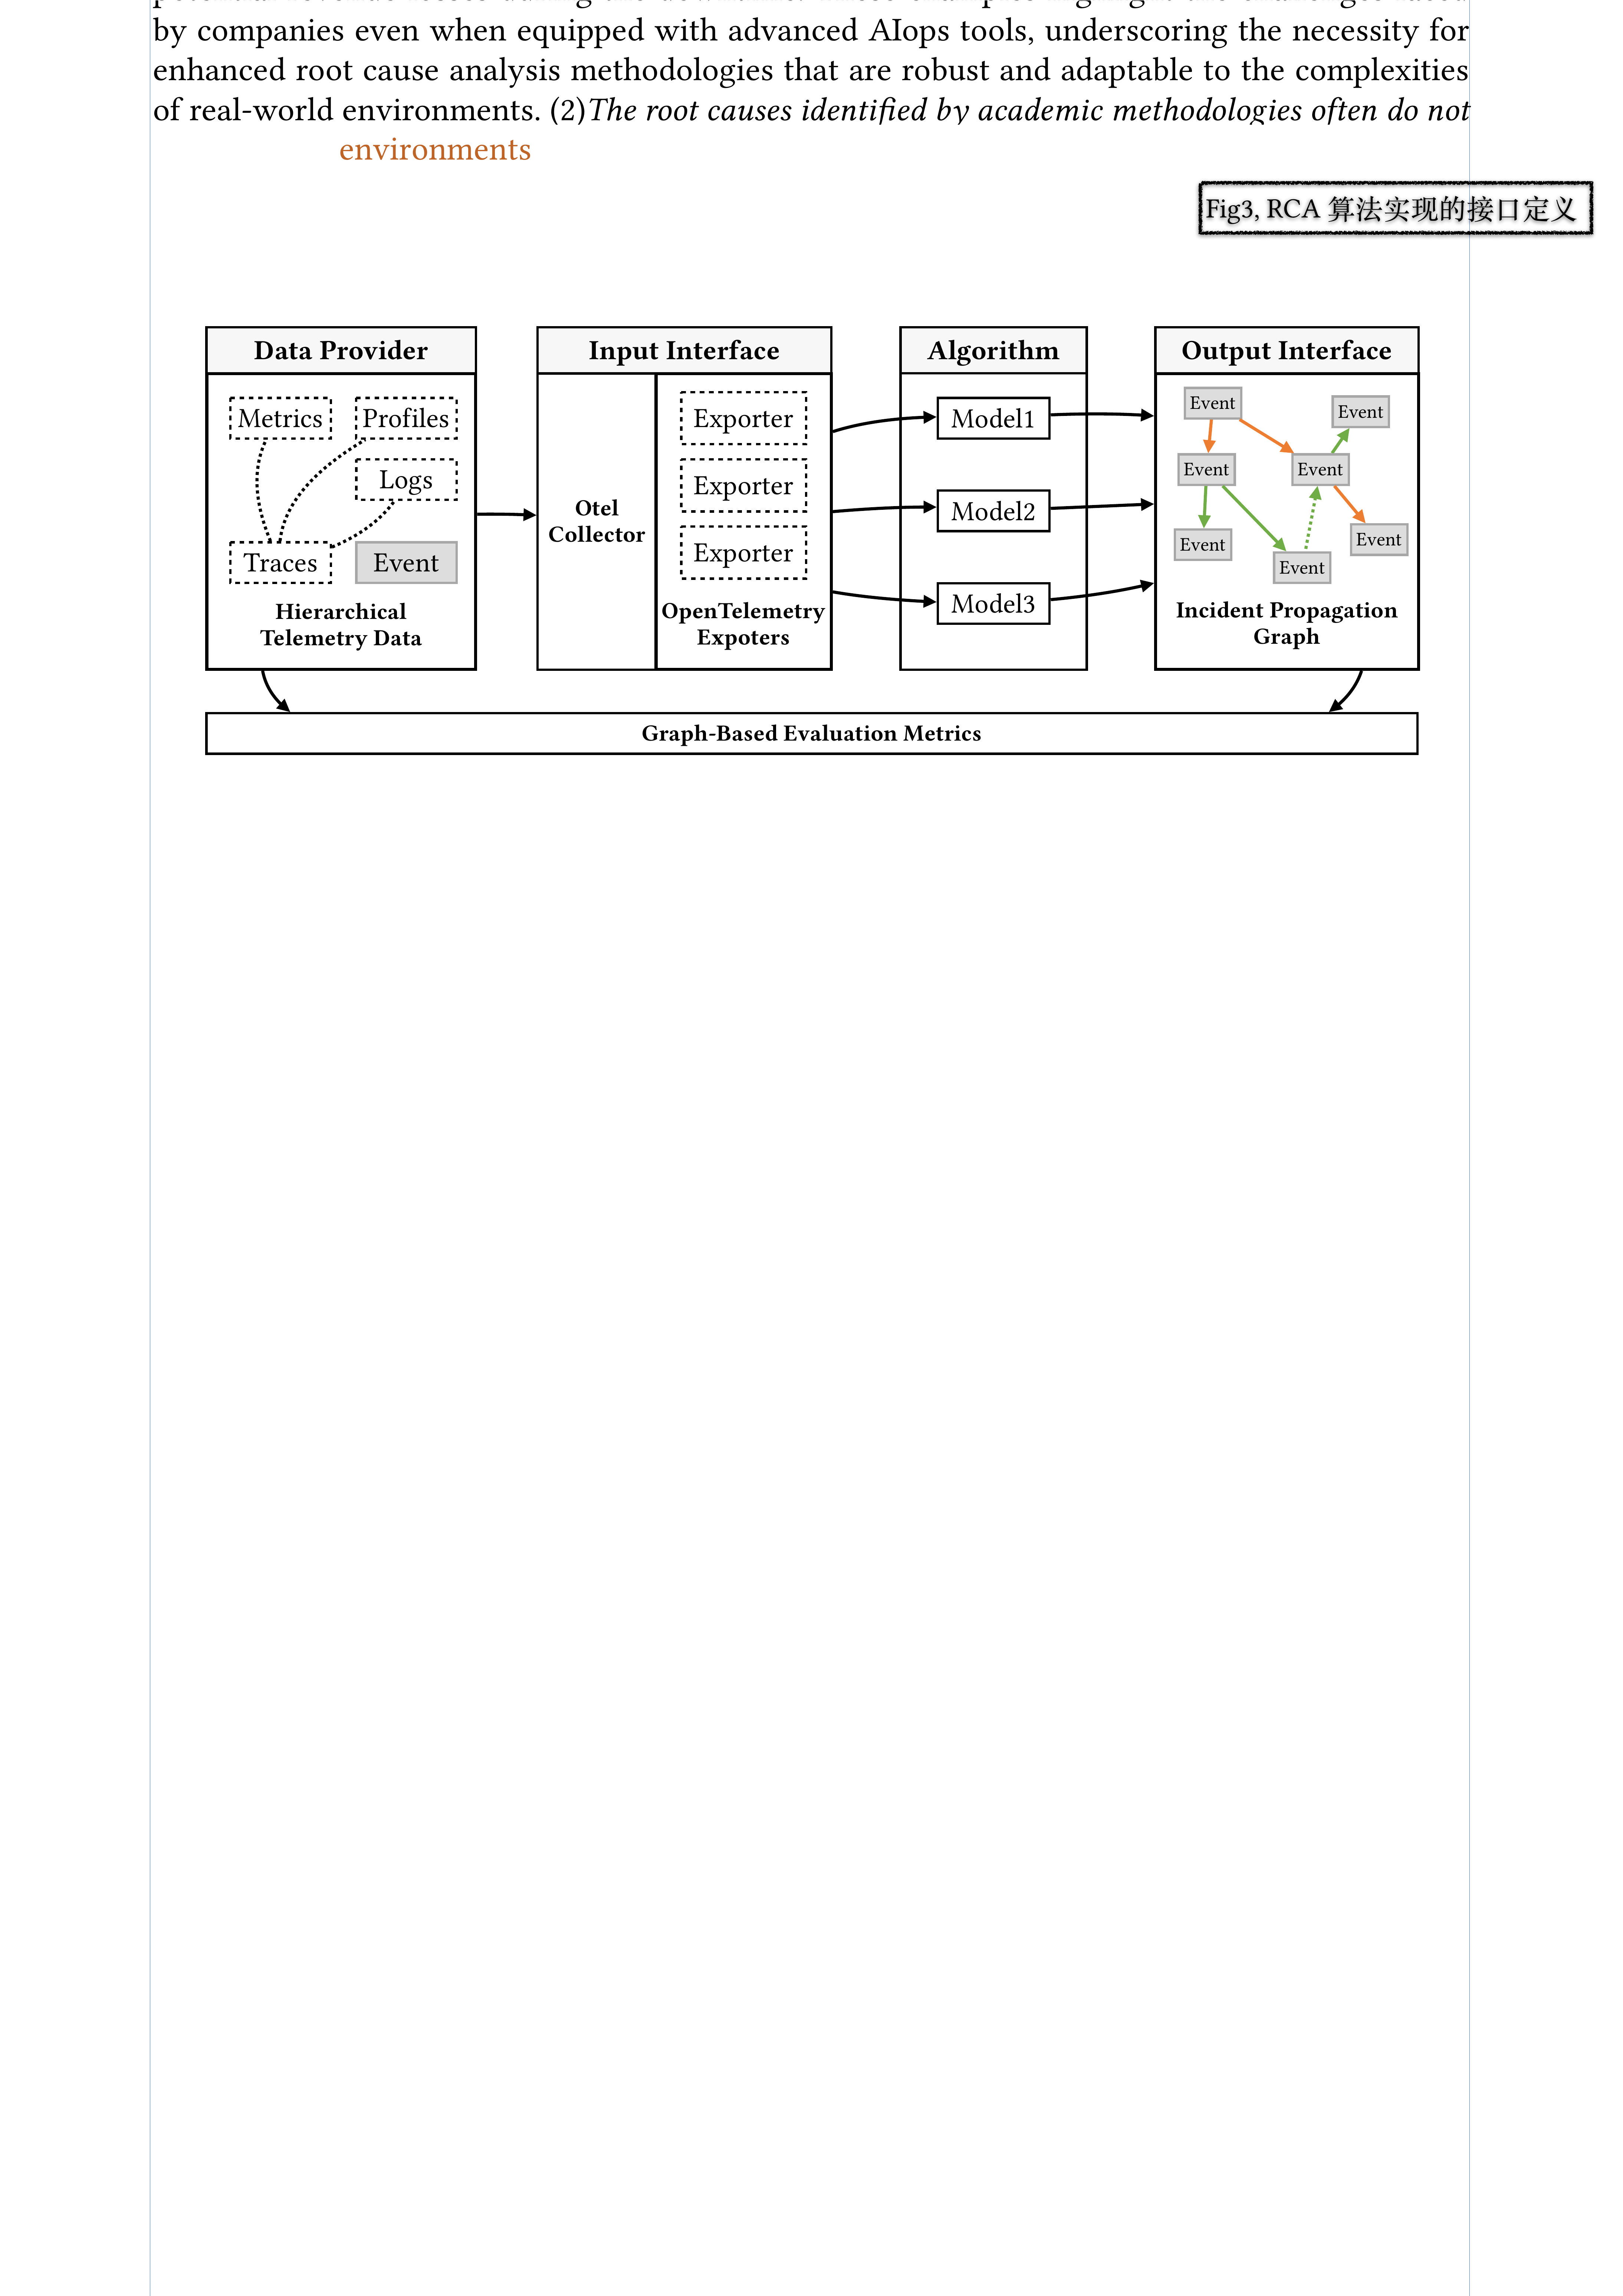}
    \caption{Typical Inference Process}
    \label{fig:processofinference}
\end{figure}

We formalize Root Cause Analysis as $\mathcal{F}: (\mathcal{O}) \rightarrow (\mathcal{G})$, where $\mathcal{O}$ denotes the hierarchical observation data, including logs, metrics, traces, events, and profiling data, $\mathcal{G}$ denotes the incident propagation graph.

\[
\mathcal{O} = \{ \mathcal{L}, \mathcal{M}, \mathcal{P},  \mathcal{T}, \mathcal{E} \}
\]

Where:
\begin{itemize}
    \item $\mathcal{L}$ denotes logs
    \item $\mathcal{M}$ denotes metrics
    \item $\mathcal{P}$ denotes profiling data
    \item $\mathcal{T}$ denotes traces
    \item $\mathcal{E}$ denotes events
\end{itemize}

In this hierarchical structure, each element of $\mathcal{O}$ captures a specific aspect of system observation data, aiding in comprehensive root cause analysis in complex systems. Specifically, as shown in the first part of Fig.~\ref{fig:processofinference}, traces act as the skeleton that associates scattered data, such as metrics, profiles, and logs. Events serve as an abstract interface that describes or summarizes anomalies in this monitoring data (detailed explanation follows). This formalization can be adapted to different scenarios, ensuring a robust approach to system monitoring and analysis.

\subsection{Logs ($\mathcal{L}$)}

Logs are recorded messages that capture the state and behavior of systems, structured into hierarchical levels:

\[
\mathcal{L} = \{ \mathcal{L}_1, \mathcal{L}_2, \ldots, \mathcal{L}_n \}
\]

Where each $\mathcal{L}_i$ represents a different level, such as:
\begin{itemize}
    \item $\mathcal{L}_c$: Component logs (e.g., container, microservice)
    \item $\mathcal{L}_s$: System logs (e.g., operating system, host)
    \item $\mathcal{L}_a$: Application logs (e.g., user applications)
    \item $\mathcal{L}_n$: Network logs (e.g., network traffic)
\end{itemize}

\subsection{Metrics ($\mathcal{M}$)}

Metrics are numerical data points that measure various aspects of system performance, also structured hierarchically:

\[
\mathcal{M} = \{ \mathcal{M}_1, \mathcal{M}_2, \ldots, \mathcal{M}_n \}
\]

Where each $\mathcal{M}_i$ represents a different level, such as:
\begin{itemize}
    \item $\mathcal{M}_r$: Resource metrics (e.g., CPU, memory, disk usage)
    \item $\mathcal{M}_s$: Service metrics (e.g., response time, throughput)
    \item $\mathcal{M}_h$: Host metrics (e.g., system load, uptime)
    \item $\mathcal{M}_a$: Application metrics (e.g., error rates, transaction rates)
\end{itemize}

\subsection{Profiling Data ($\mathcal{P}$)}

Profiling data provides insights into the performance characteristics of code execution:

\[
\mathcal{P} = \{ \mathcal{P}_1, \mathcal{P}_2, \ldots, \mathcal{P}_n \}
\]

Where each $\mathcal{P}_i$ represents a different type of profiling data:
\begin{itemize}
    \item $\mathcal{P}_c$: CPU profiling (e.g., CPU usage by function)
    \item $\mathcal{P}_m$: Memory profiling (e.g., memory allocation, leaks)
    \item $\mathcal{P}_i$: I/O profiling (e.g., disk, network I/O)
    \item $\mathcal{P}_t$: Time profiling (e.g., execution time, latency)
\end{itemize}

\subsection{Traces ($\mathcal{T}$)}

Traces track the flow of requests through various components of a system, linking logs and metrics across different levels:

\[
\mathcal{T} = \{ \mathcal{T}_1, \mathcal{T}_2, \ldots, \mathcal{T}_n \}
\]

Where each $\mathcal{T}_i$ represents trace data at different levels:
\begin{itemize}
    \item $\mathcal{T}_r$: Request traces (e.g., API calls, user transactions)
    \item $\mathcal{T}_d$: Dependency traces (e.g., microservices interactions)
    \item $\mathcal{T}_f$: Function traces (e.g., execution of specific functions or methods)
\end{itemize}

\subsection{Events ($\mathcal{E}$)}

Events capture discrete changes or occurrences within the system, aggregated into different categories:

\[
\mathcal{E} = \{ \mathcal{E}_1, \mathcal{E}_2, \ldots, \mathcal{E}_n \}
\]

Where each $\mathcal{E}_i$ represents a different type of event:
\begin{itemize}
    \item $\mathcal{E}_c$: Configuration events (e.g., configuration changes)
    \item $\mathcal{E}_d$: Deployment events (e.g., new deployments, updates)
    \item $\mathcal{E}_u$: Usage events (e.g., user behavior, traffic spikes)
    \item $\mathcal{E}_f$: Failure events (e.g., errors, crashes)
\end{itemize}

An event is an interface (abstract class) that describes a change. A typical event contains details about what changed, where it changed, when it happened, and who or what caused the change. For instance, configuration events describe who made the change and where it occurred. Similarly, failure events indicate that the error rate exceeded 20\% at a certain time in a specific service.

Thus we further define $\mathcal{E}_i$ as:

\[
\mathcal{E}_i = \{ t_i, a_i, u_i, l_i \}
\]

Where:

\begin{enumerate}
    \item $t_i \in \mathbb{T}$ is the timestamp of the event.
    \item $a_i \in \mathbb{A}$ is the action or change described by the event.
    \item $u_i \in \mathbb{U}$ is the entity responsible for the event.
    \item $l_i \in \mathbb{L}$ is the location or context within the system.
\end{enumerate}

An Event describes or summarizes the ''change'' in the system. In other words, ''describe'' means the event is straightforward, like a deployment operation, containing where, when, what, and who; ''summarize'' indicates that there needs some transformation from the raw information, i.e., previously mentioned Log, Trace, Metric, Profiling. With some ''Anomaly Detection'' methods (which are called alerts in the industry), these raw telemetry data can be transformed into more abstract information: events.

\subsection{Incident Propagation Graph $\mathcal{G}$}

Let $\mathcal{E}$ be the set of all events, where each event $e \in \mathcal{E}$ is defined as $\mathcal{E}_i = \{ t_i, a_i, u_i, l_i \}$. The Incident Propagation Graph $\mathcal{G}$ is then defined as:

\[
\mathcal{G} = (\mathcal{V}, \mathcal{R})
\]

where:
\begin{itemize}
\item $\mathcal{V}$ is the set of vertices representing the events, i.e., $\mathcal{V} = { e \in \mathcal{E} }$.
\item $\mathcal{R}$ is the set of directed edges representing the relationships between events. Each relation $r_{uv} \in \mathcal{R}$ indicates a relationship from event $u$ to event $v$.
\end{itemize}

For each edge $r_{uv}$:
\begin{itemize}
\item $r$ means one event is another event's root cause.
\item $t$ means one event is another event's trigger.
\end{itemize}

The relationship $r$ and $t$ indicates the causal influence of each corresponding event. In other words, an incident propagation chain can be described as a quintuple, $\mathcal{C} = (e_{rc}, e_{tr}, e_{re}, r_{r}, r_{t})$, where $e_{rc}$ means the root cause event, $e_{tr}$ means the trigger event, $e_{re}$ means the result event, and $r_{r}, r_{t}$ represent the relationships between these three events. These two relations have the same chain ID, binding themselves together.

$\mathcal{G}$ models the interactions and dependencies between events, helping to identify which events are root causes, triggers, and results. This formalization aids in visualizing and understanding the propagation of incidents across the system. Specifically, the distinction between "root cause" and "trigger" is important because, in practice, the first priority is to stop the incident from propagating to other services or minimize economic and reputational losses (the "trigger"). After containment, the ultimate "root cause" (which may be a code bug, configuration issue, or design flaw) is identified to prevent the recurrence of the incident.

A clear definition of the RCA output can further help developers or automatic mitigation strategies perform better. Once they find the "narrow waist" of the incidents, they can easily stop the propagation. Additionally, the graph of events can provide an easier interpretation of the incident, giving more confidence to the SRE.

\section{HIERARCHICAL EVALUATION METRIC}

% 关于metric
% 1. ground truth怎么设置。现在的输入是层次化的telemetry数据；算法的第一步任务是把观测数据转换成event，第二步是把event构建成一个相对完整的event graph。从评估的角度来说，我们不应该关心算法具体是怎么实现的，而是只能关心算法最后输出的结果。而算法输出的结果，最后就是一个event graph。这里的任务就变成了，怎么根据输入的数据，来构造一个ground truth的event graph。但这很难，因为我们只知道故障是在哪里注入的，注入的故障类型是什么，注入的量级是多少；而不知道故障究竟是怎么传播的，什么程度下才能定义为故障。换句话说，想要根据注入的故障来知道故障的传播路径，这个有点像污点分析，但问题是这类微服务不像是代码一样有严格的调用、依赖关系可以查询，而只有一些笼统的，例如trace、或者是服务本身的静态依赖、服务和基础设施的静态架构等。如何从这些现有信息中提出ground truth的传播路径还是个大问题。
% 但是！虽然构建一个通用的链路传播ground truth很难，但是我们在这个survey里不需要实现，我们可以假设所有的相关信息都是存在的，然后根据这些信息抽象成符号，然后提出一个metric即可。

Based on the definition provided above, we developed hierarchical evaluation metrics to assess the performance of various models. As illustrated in Fig.~\ref{fig:hierarchicalmetric}, our approach includes metrics for event similarity, event chain similarity, event set similarity, and event graph similarity.
We begin by defining the similarity of the smallest unit, the event, and then build upon this to define the similarity of event chains and event sets. Finally, we establish the event graph similarity based on the similarity of event chains. It is important to note that while we provide general metrics for evaluating event similarity, these metrics should be adapted to specific datasets. However, the overall methodology remains consistent.

\begin{figure}[t]
    \centering
    \includegraphics[width=1\linewidth]{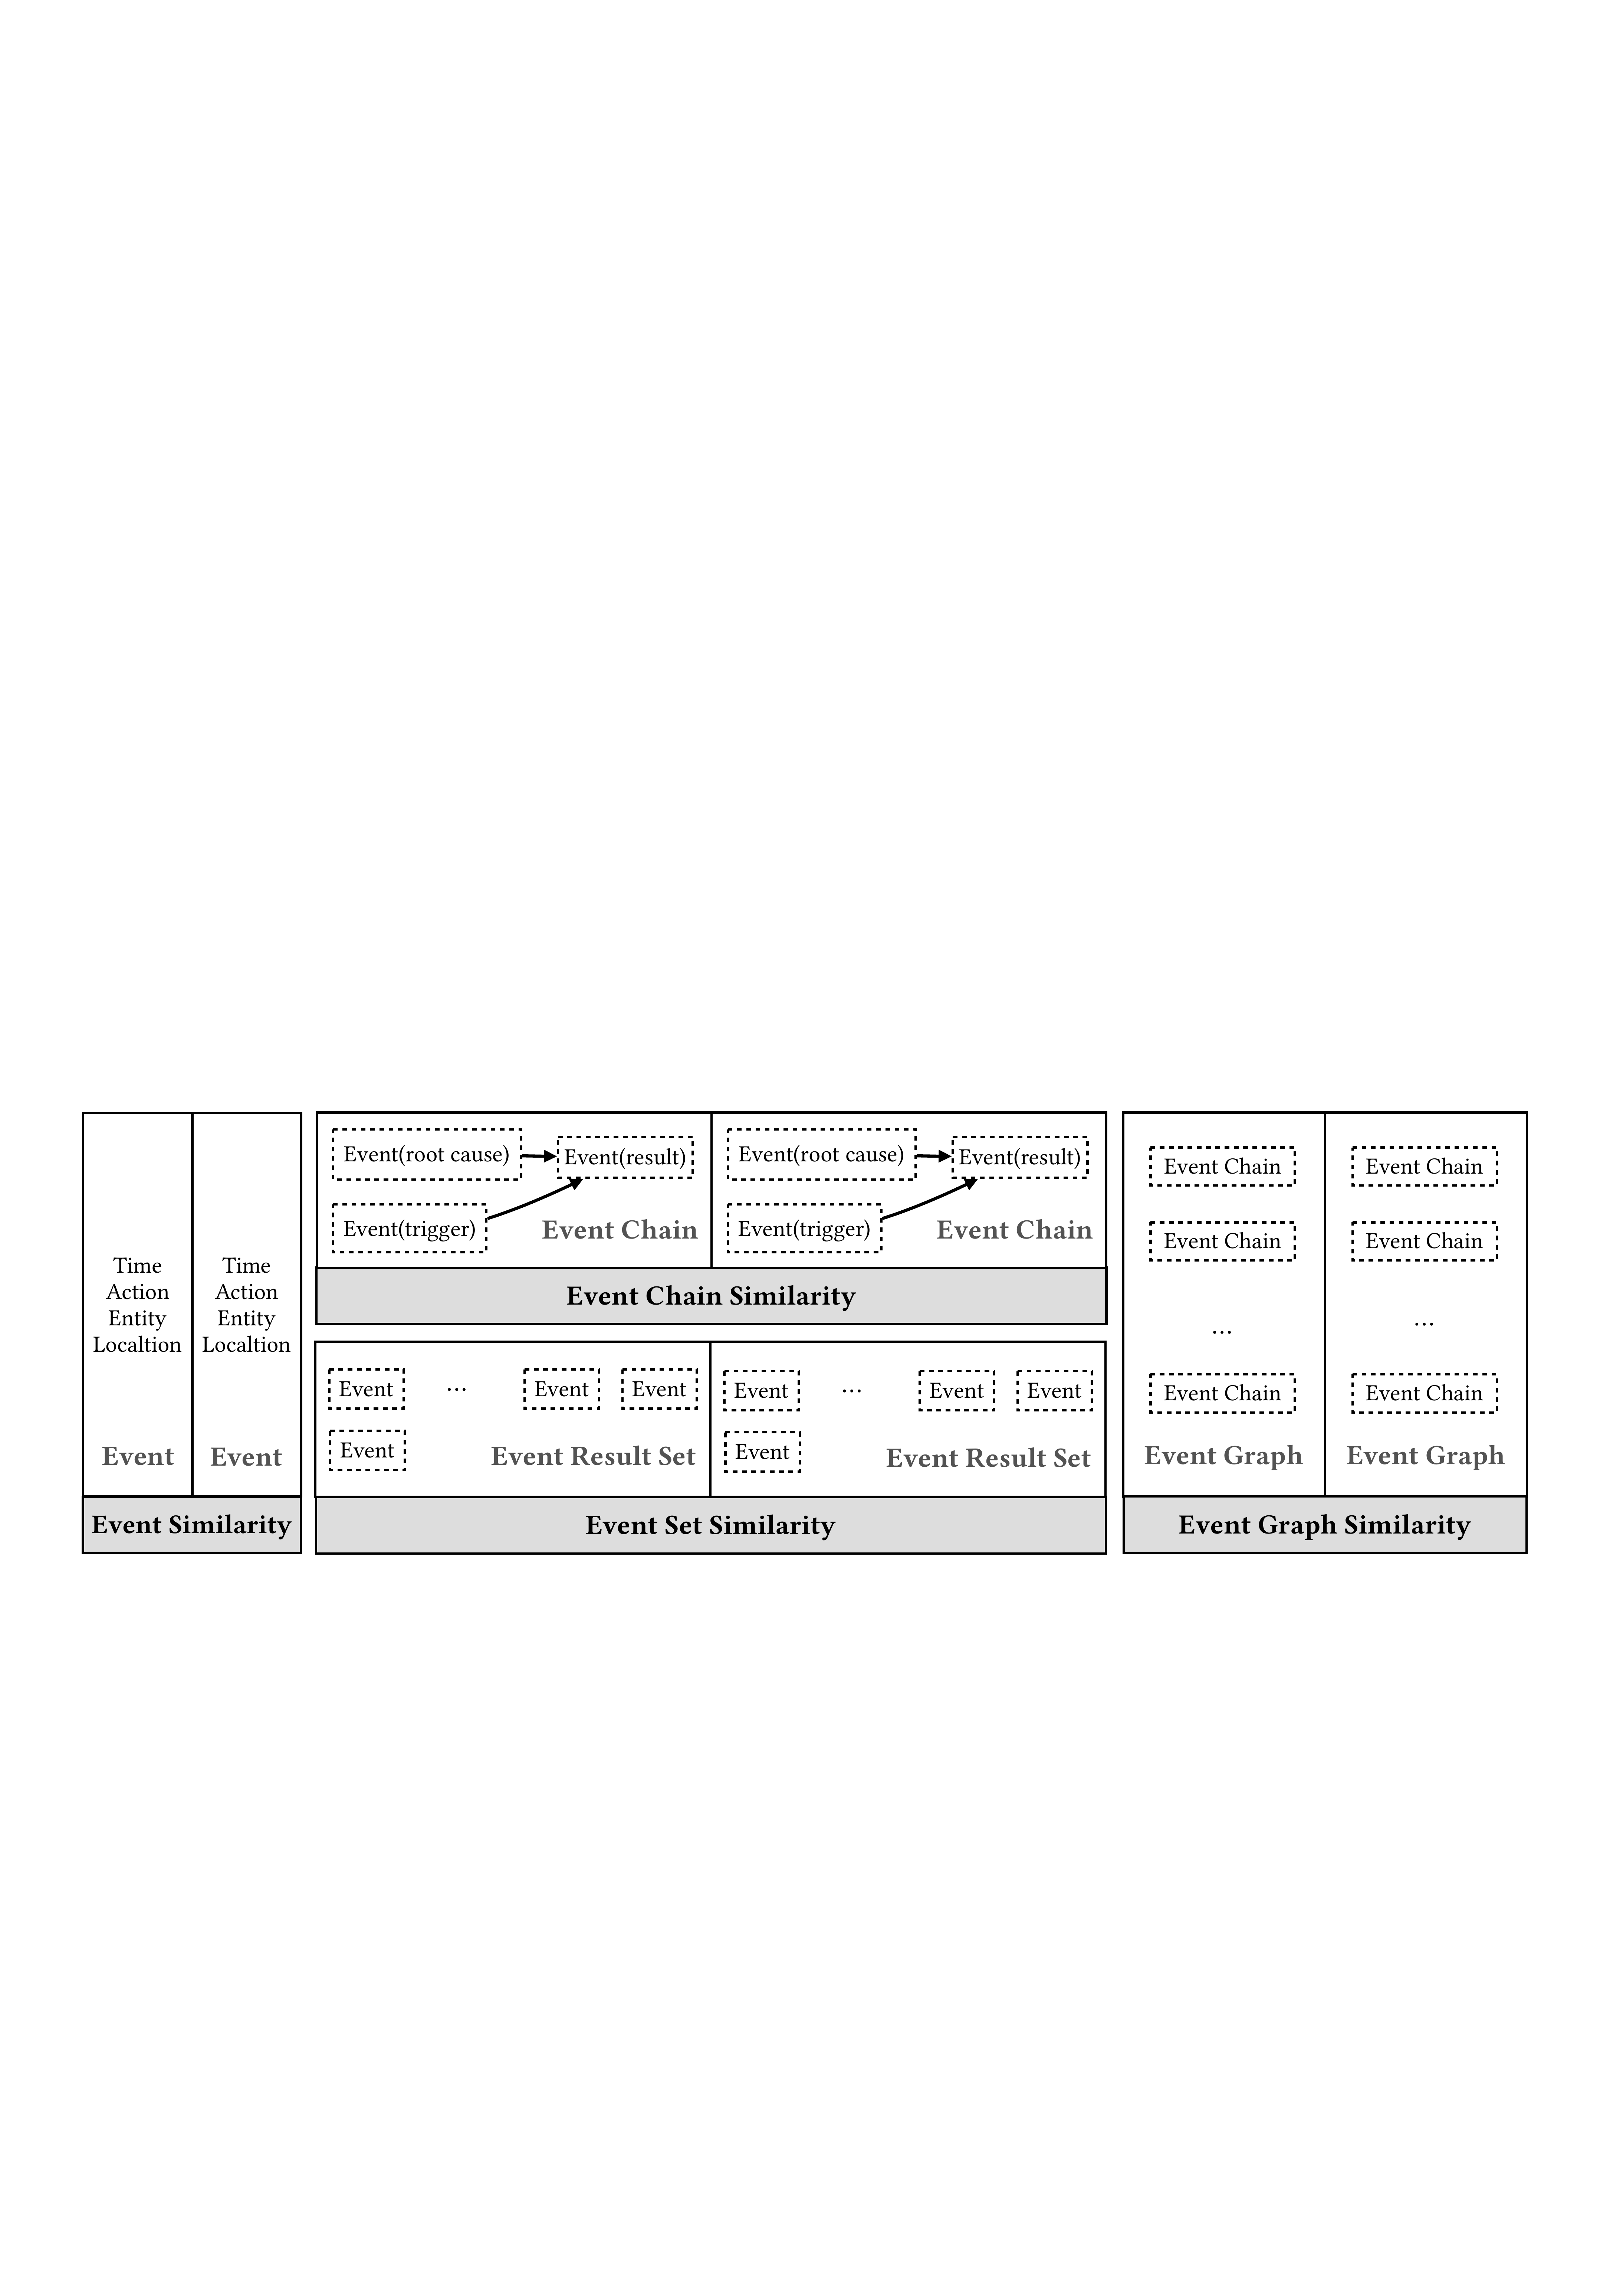}
    \caption{Hierarchical Evaluation Metrics}
    \label{fig:hierarchicalmetric}
\end{figure}

\subsection{Event Similarity}

To compute the similarity between two events, $\mathcal{E}_i$ and $\mathcal{E}_j$, need to define a similarity metric that considers the different components of an event: timestamp, action, entity, and location. Here's a possible similarity calculation formula:

\[
\text{Sim}(\mathcal{E}_i, \mathcal{E}_j) = \alpha \cdot \text{Sim}_t(t_i, t_j) + \beta\cdot \text{Sim}_a(a_i, a_j)+\gamma\cdot \text{Sim}_u(u_i, u_j) + \delta\cdot \text{Sim}_l(l_i, l_j)
\]

where:
\begin{itemize}
    \item $\text{Sim}_t(t_i, t_j)$ is the similarity between the timestamps $t_i$ and $t_j$. This can be computed using a time-based function such as the inverse of the absolute time difference, normalized to a range $[0, 1]$. \[
\text{Sim}_t(t_i, t_j) = exp(-\frac{|t_i-t_j|}{\tau})
\] $\tau$ is a time decay constant.

    \item $\text{Sim}_a(a_i, a_j)$ is the similarity between the actions $a_i$ and $a_j$. This can be computed using a semantic similarity measure such as cosine similarity if the actions are represented as vectors (e.g., using word embeddings). \[
    \text{Sim}_a(a_i,a_j)=\text{cosine\_similarity}(v(a_i),v(a_j))
    \] Here, $v(a_i)$and $v(a_j)$ are vector representations of actions $a_i$ and $a_j$.
    
    \item $\text{Sim}_u(u_i, u_j)$ is the similarity between the entities $u_i$ and $u_j$. This can be a binary similarity (1 if they are the same entity, 0 otherwise) or a more sophisticated measure if the entities have additional attributes. \[
        \text{Sim}_u(u_i, u_j) = \begin{cases} 
        1 & \text{if } u_i = u_j \\
        0 & \text{otherwise}
        \end{cases}
    \]
    
    \item $\text{Sim}_l(l_i, l_j)$ is the similarity between the locations $l_i$ and $l_j$. This can be computed using a spatial similarity measure if the locations are spatial coordinates or using a categorical similarity if the locations are predefined categories, for example, the service dependency graph.
    \[
        \text{Sim}_l(l_i,l_j)=\text{location\_similarity}(l_i,l_j)
    \]
        
    \item $\alpha,\beta,\gamma$ and $\delta$ are weights that 
    sum to 1 ($\alpha+\beta+\gamma+\delta=1$)and reflect the relative importance of each component in the overall similarity measure. 

\end{itemize}

\subsection{Event Set Similarity Metric}

To compute the similarity between two sets of events, $\mathcal{E}_A$ and $\mathcal{E}_B$, we define an Event Set Similarity Metric (ESSM). This metric aggregates the pairwise similarities of events within the sets into a single similarity score. We describe several approaches for this aggregation:

\paragraph{1. Average Maximum Similarity (AMS)}
For each event in one set, find the most similar event in the other set and compute the average of these maximum similarities.

\[
\text{AMS}(\mathcal{E}_A, \mathcal{E}_B) = \frac{1}{2} \left( \frac{1}{|\mathcal{E}_A|} \sum_{e_A \in \mathcal{E}_A} \max_{e_B \in \mathcal{E}_B} \text{Sim}(e_A, e_B) + \frac{1}{|\mathcal{E}_B|} \sum_{e_B \in \mathcal{E}_B} \max_{e_A \in \mathcal{E}_A} \text{Sim}(e_A, e_B) \right)
\]

\paragraph{2. Hausdorff Similarity Metric (HSM)}
This metric is based on the Hausdorff distance, measuring the greatest of all the minimum distances from any point in one set to the nearest point in the other set, using similarity as the inverse of distance.

\[
\text{HSM}(\mathcal{E}_A, \mathcal{E}_B) = \max \left( \max_{e_A \in \mathcal{E}_A} \min_{e_B \in \mathcal{E}_B} (1 - \text{Sim}(e_A, e_B)), \max_{e_B \in \mathcal{E}_B} \min_{e_A \in \mathcal{E}_A} (1 - \text{Sim}(e_A, e_B)) \right)
\]

\paragraph{3. Overall Maximum Similarity (OMS)}
Calculate the average similarity of all possible pairs of events between the two sets.

\[
\text{OMS}(\mathcal{E}_A, \mathcal{E}_B) = \frac{1}{|\mathcal{E}_A| \cdot |\mathcal{E}_B|} \sum_{e_A \in \mathcal{E}_A} \sum_{e_B \in \mathcal{E}_B} \text{Sim}(e_A, e_B)
\]

\paragraph{4. Simplified Average Maximum Similarity (SAMS)}
For each event in one set, find the most similar event in the other set, then compute the average of these maximum similarities, considering both directions.

\[
\text{SAMS}(\mathcal{E}_A, \mathcal{E}_B) = \frac{1}{|\mathcal{E}_A| + |\mathcal{E}_B|} \left( \sum_{e_A \in \mathcal{E}_A} \max_{e_B \in \mathcal{E}_B} \text{Sim}(e_A, e_B) + \sum_{e_B \in \mathcal{E}_B} \max_{e_A \in \mathcal{E}_A} \text{Sim}(e_A, e_B) \right)
\]

\subsection{Incident Propagation Chain Similarity}

Previously, we defined Incident Propagation Chain can be described as a quintuple, $\mathcal{C} = (e_{rc}, e_{tr}, e_{re}, r_{r}, r_{t})$. We also defined how to calculate event similarity, here we introduce how to calculate the chain similarity since the chain is the basic unit of the graph.

To compute the similarity between two incident propagation chains, we need to consider the similarity between the root cause events, trigger events, result events, and their relationships. Given that an incident propagation chain is described as a quintuple $\mathcal{C} = (e_{rc}, e_{tr}, e_{re}, r_{r}, r_{t})$, we define the similarity between two incident propagation chains $\mathcal{C}_1 = (e_{rc_1}, e_{tr_1}, e_{re_1}, r_{r_1}, r_{t_1})$ and $\mathcal{C}_2 = (e_{rc_2}, e_{tr_2}, e_{re_2}, r_{r_2}, r_{t_2})$ as follows:

\[
\text{Sim}(\mathcal{C}_1, \mathcal{C}_2) = \lambda_1 \cdot \text{Sim}(\mathcal{E}_{rc_1}, \mathcal{E}_{rc_2}) + \lambda_2 \cdot \text{Sim}(\mathcal{E}_{tr_1}, \mathcal{E}_{tr_2}) + \lambda_3 \cdot \text{Sim}(\mathcal{E}_{re_1}, \mathcal{E}_{re_2}) + \lambda_4 \cdot \text{Sim}(r_{r_1}, r_{r_2}) + \lambda_5 \cdot \text{Sim}(r_{t_1}, r_{t_2})
\]

where:
\begin{itemize}
    \item $\text{Sim}(\mathcal{E}_{rc_1}, \mathcal{E}_{rc_2})$ is the similarity between the root cause events, calculated using the previously defined event similarity formula.
    \item $\text{Sim}(\mathcal{E}_{tr_1}, \mathcal{E}_{tr_2})$ is the similarity between the trigger events, calculated using the previously defined event similarity formula.
    \item $\text{Sim}(\mathcal{E}_{re_1}, \mathcal{E}_{re_2})$ is the similarity between the result events, calculated using the previously defined event similarity formula.
    \item $\text{Sim}(r_{r_1}, r_{r_2})$ is the similarity between the root cause relationships, which can be defined as binary similarity (1 if the relationships are the same, 0 otherwise).
    \item $\text{Sim}(r_{t_1}, r_{t_2})$ is the similarity between the trigger relationships, which can be defined as binary similarity (1 if the relationships are the same, 0 otherwise).
    \item $\lambda_1, \lambda_2, \lambda_3, \lambda_4, \lambda_5$ are weights that sum to 1 ($\lambda_1 + \lambda_2 + \lambda_3 + \lambda_4 + \lambda_5 = 1$) and reflect the relative importance of each component in the overall similarity measure.
\end{itemize}

This formula comprehensively considers the similarities between events and the relationships between them, thereby accurately measuring the similarity between two incident propagation chains.

\subsection{Similarity of Event Graph(Incident Propagation Graph)}

An event graph contains nodes (events) and edges (relations). To compare the similarity of event graphs, we can use the similarity of incident propagation chains as the basic unit of the graph. Given two incident propagation graphs $\mathcal{G}_1 = (\mathcal{V}_1, \mathcal{R}_1)$ and $\mathcal{G}_2 = (\mathcal{V}_2, \mathcal{R}_2)$, we define the graph similarity as follows:

\[
\text{Sim}(\mathcal{G}_1, \mathcal{G}_2) = \frac{1}{|\mathcal{C}_1| \cdot |\mathcal{C}_2|} \sum_{i=1}^{|\mathcal{C}_1|} \sum_{j=1}^{|\mathcal{C}_2|} \text{Sim}(\mathcal{C}_{1i}, \mathcal{C}_{2j})
\]

where:
\begin{itemize}

    \item $\mathcal{C}_1$ and $\mathcal{C}_2$ are the sets of incident propagation chains in graphs $\mathcal{G}_1$ and $\mathcal{G}_2$, respectively.
    \item $|\mathcal{C}_1|$ and $|\mathcal{C}_2|$ are the numbers of chains in graphs $\mathcal{G}_1$ and $\mathcal{G}_2$.
    \item $\text{Sim}(\mathcal{C}_{1i}, \mathcal{C}_{2j})$ is the similarity between the $i$-th chain in $\mathcal{G}_1$ and the $j$-th chain in $\mathcal{G}_2$, calculated using the previously defined chain similarity formula.

\end{itemize}
This formula calculates the average similarity between all pairs of chains from the two graphs, providing a comprehensive measure of the overall similarity between the incident propagation graphs.
